# Supplementary material for: How Much is Performance Worth to Users? A Quantitative Approach
Source: arXiv:2204.13698 source file (2022-04-27)
Supplement: Supplementary file 1 [file appendix_a.tex]

\section*{Appendix A} \label{appendix:a}

This appendix provides details.

\subsection{Tasks}

The three tasks asked of participants are as follows:
(Differences between the three tasks are delineated by slashes.)
\begin{displayquote}
    \begin{enumerate}
    \item Open up Microsoft Word.
    \item Create a new Word document titled ``Task 1''/``Task 2''/``Task 3''.
    \item Open up Google Maps in a web browser. Find out long it would take to drive from Los Angeles, USA to New York, USA/from Casablanca, Morocco to Cairo, Egypt/from Sydney, Australia to Perth, Australia. Write down this number in the previously created Word document.
    \item Open an image search engine in a new tab. Find a photo of the Statue of Liberty/the Eiffel Tower/the Pyramids of Giza and copy the photo into the Word document.
    \item Open YouTube in a new tab. Find a video of a live performance of the classical music piece ``Bolero'' by Maurice Ravel/``Rhapsody in Blue'' by George Gershwin/``Fantasia on a Theme by Thomas Tallis'' by Ralph Vaughn Williams. Copy and paste the video's URL into the Word document.
    \item Save the Word document as a PDF.
    \item Upload the PDF to a web server via a provided webpage
    \item Close all tabs and delete the previously created Word document and PDF.
\end{enumerate}
\end{displayquote}

\subsection{Noticability of Slowdowns}

\begin{displayquote}
    ``Your computer may have been slowed down during either Task 2 or Task 3. We will now ask you to pick during which (if any) of the tasks your computer was slowed down. Only one of the answers below is correct. To incentivize you to answer to the best of your ability, we will award you a bonus of \$0.25 if you choose correctly.''
    \end{displayquote}
    
    Participants are then asked to choose from one of the following three options:
    
    \begin{displayquote}
    \begin{itemize}
        \item ``My computer was running slower during Task~2 than during Task~3''
        \item ``My computer was running slower during Task~3 than during Task~2''
        \item ``My computer was running at same speed during Task~2 and Task~3''
    \end{itemize}
    \end{displayquote}
    
    To eliminate the possibility of any ordering effects of the above three options, the program randomizes the order of the above three options.
