# Supplementary material for: How Much is Performance Worth to Users? A Quantitative Approach
Source: arXiv:2204.13698 source file (2022-04-27)
Supplement: Supplementary file 2 [file appendix_b.tex]

\section*{Appendix B} \label{appendix:b}
